# Supplementary material for: On Preempting Advanced Persistent Threats Using Probabilistic Graphical Models
Source: arXiv:1903.08826 source file (2019-03-21)
Supplement: Supplementary file 1 [file appendix.tex]

\newpage
\pagebreak
\appendices
